# Supplementary material for: A Novel Evaluation Perspective on GNNs-based Recommender Systems through the Topology of the User-Item Graph
Source: arXiv:2408.11762 source file (2024-08-21)
Supplement: Supplementary file 1 [file appendix.tex]

\section{Appendix}

\subsection{Classical dataset characteristics}
\label{app:class_charact}

We provide a brief overview of popular classical characteristics describing a recommendation dataset (as presented in~\cite{DBLP:journals/tmis/AdomaviciusZ12, DBLP:conf/sigir/DeldjooNSM20}). Regarding the adopted notation, we assume the reader is aware of the background from Section \ref{sec:topological-characteristics}.

\subsubsection{Space size} The space size estimates the number of all possible interactions that might exist among users and items:

\begin{equation}
    \zeta = \sqrt{UI}.
\end{equation}

\subsubsection{Shape} The shape of a recommendation dataset is defined as the ratio between the number of users and items:

\begin{equation}
    \pi = \frac{U}{I}.
\end{equation}

\subsubsection{Density} The density of a recommendation dataset measures the ratio of actual user-item interactions with respect to all possible interactions that might connect all users and items:

\begin{equation}
    \delta = \frac{E}{UI},
\end{equation}
where $E = |\{(u, i)\;|\;\mathbf{R}_{u, i} = 1\}|$ is the number of interactions existing among users and items in the recommendation data.

\subsubsection{Gini coefficient} 
\label{sec:gini}
The Gini coefficient is an estimation of the interactions' concentration for both users and items. When calculated on $\mathcal{U}$ and $\mathcal{I}$, we have:
\begin{equation}
    \kappa_{\mathcal{U}} = \frac{\sum\limits_{u = 1}^{U-1}\sum\limits_{v = u + 1}^{U}abs(\sigma_u - \sigma_v)}{U\sum\limits_{u = 1}^{U}\sigma_u},
    \qquad \kappa_{\mathcal{I}} = \frac{\sum\limits_{i = 1}^{I-1}\sum\limits_{j = i + 1}^{I}abs(\sigma_i - \sigma_j)}{I\sum\limits_{i = 1}^{I}\sigma_i}, 
\end{equation}
where $abs()$ is the function returning the absolute value. 

\subsection{(Extended) Topological characteristics in graph collaborative filtering}
\label{app:graph-recsys}
In this section, we present the four selected graph-based recommender systems used in our analysis, and re-formulate their techniques to make the \textit{topological} data characteristics explicitly emerge. As additional background with respect to Section \ref{sec:topological-characteristics}, we introduce the notations $\mathbf{e}_u \in \mathbb{R}^b$ and $\mathbf{e}_i \in \mathbb{R}^b$ as the initial embeddings of the nodes for user $u$ and item $i$, respectively, where $b << U, I$. Then, in the case of message-propagation at different layers, we also introduce the notations $\mathbf{e}_u^{(l)}$ and $\mathbf{e}_i^{(l)}$ to indicate the updated node embeddings for user $u$ and item $i$ after $l$ propagation layers, with $0 \leq l \leq L$ (note that $\mathbf{e}_u^{(0)} = \mathbf{e}_u$ and $\mathbf{e}_i^{(0)} = \mathbf{e}_i$).

\subsubsection{LightGCN} \citet{DBLP:conf/sigir/0001DWLZ020} propose to lighten the graph convolutional layer presented in~\citet{DBLP:conf/iclr/KipfW17} for the recommendation task. Specifically, their layer removes feature transformation and non-linearities:
\begin{equation}
\label{eq:lightgcn}
    \mathbf{e}_u^{(l)} = \sum\limits_{i' \in \mathcal{N}_u^{(1)}} \frac{A_{ui'} \mathbf{e}_{i'}^{(l - 1)}}{\sqrt{\sigma_u  \sigma_{i'}}}, \quad \mathbf{e}_i^{(l)} = \sum\limits_{u' \in \mathcal{N}_i^{(1)}} \frac{A_{iu'} \mathbf{e}_{u'}^{(l - 1)}}{\sqrt{\sigma_i \sigma_{u'}}},
\end{equation}
where each neighbor contribution is weighted through the corresponding entry in the normalized Laplacian adjacency matrix to flatten the differences among nodes with high and low degrees. Since $A_{ui'} = 1, \text{ } \forall i' \in \mathcal{N}^{(1)}_u$ (the dual holds for $A_{iu'}$), the contribution weighting comes only from the denominator.  

\subsubsection{DGCF} \citet{DBLP:conf/sigir/WangJZ0XC20} assume that user-item interactions are decomposed into a set of independent intents, representing the specific aspects users may be interested in when interacting with items. In this respect, the authors propose to iteratively learn a set of weighted adjacency matrices $\{\mathbf{\tilde{A}}_1, \mathbf{\tilde{A}}_2, \dots\}$, where each of them records the user-item importance weights based on the specific intent it represents. Then, they introduce a graph disentangling layer for each weighted adjacency matrix:
\begin{equation}
    \mathbf{e}_{u, *}^{(l)} = \sum\limits_{i' \in \mathcal{N}_u^{(1)}} \frac{\tilde{A}_{ui', *} \mathbf{e}_{i', *}^{(l - 1)}}{\sqrt{\sigma_{u, *} \sigma_{i', *}}}, \quad \mathbf{e}_{i, *}^{(l)} = \sum\limits_{u' \in \mathcal{N}_i^{(1)}} \frac{\tilde{A}_{iu', *} \mathbf{e}_{u', *}^{(l - 1)}}{\sqrt{\sigma_{i, *} \sigma_{u', *}}},
\end{equation}
where $\tilde{A}_{ui', *}$ and $\mathbf{e}_{i',*}^{(l-1)}$ are the learned importance weight of user $u$ on item $i'$ and the embedding of item $i'$ for any intent, while $\sigma_{u,*}$ is the corresponding node degree calculated on $\mathbf{\tilde{A}_{*}}$ (the same applies for the item side).    

\subsubsection{UltraGCN} \citet{DBLP:conf/cikm/MaoZXLWH21} recognize three major limitations in GCN-based message-passing for collaborative filtering, namely, (i) the asymmetric weight assignment to connected nodes when considering user-user and item-item relationships; (ii) the impossibility to diversify the importance of each type of relation (i.e., user-item, user-user, item-item) during the message-passing; (iii) the over-smoothing effect when stacking more than 3 layers. To tackle such issues, the authors propose to go beyond the traditional concept of explicit message-passing, and approximate the infinite-layer message-passing through the following:
\begin{equation}
    \mathbf{e}_u = \sum\limits_{i' \in \mathcal{N}_u^{(1)}} \frac{A_{ui'} \sqrt{\sigma_u + 1} \mathbf{e}_{i'}}{\sigma_u \sqrt{\sigma_{i'} + 1}}, \quad
    \mathbf{e}_i = \sum\limits_{u' \in \mathcal{N}_i^{(1)}} \frac{A_{iu'} \sqrt{\sigma_i + 1} \mathbf{e}_{u'}}{\sigma_{i} \sqrt{\sigma_{u'} + 1}}.
\end{equation}
Note that the procedure is not repeated for layers $l > 1$, as the method surpasses the concept of iterative message-passing. During the optimization, the model first minimizes a constraint loss that adopts negative sampling to limit the over-smoothing effect:
\begin{equation}
    \begin{aligned}
    \min\limits_{\mathbf{e}_u, \mathbf{e}_i, \mathbf{e}_j} \text{ }&-  \sum\limits_{(u,i) \in \mathbf{R}_s^{+}}\frac{1}{\sigma_u} \frac{\sqrt{\sigma_u + 1}}{\sqrt{\sigma_i + 1}} log(sig(\mathbf{e}_u^\top \cdot \mathbf{e}_i)) \text{ }+ \\
    & - \sum\limits_{(u, j) \in \mathbf{R}_s^{-}} \frac{1}{\sigma_u} \frac{\sqrt{\sigma_u + 1}}{\sqrt{\sigma_j + 1}} log(sig(-\mathbf{e}_u^\top \cdot \mathbf{e}_j)),
    \end{aligned}
\end{equation}
where $\mathbf{R}_s^{+}$ and $\mathbf{R}^{-}_s$ are pairs of positive and negative interactions sampled from the user-item matrix $\mathbf{R}$, while $log()$ and $sig()$ are the logarithm and sigmoid function. Then, they also take into account the item-projected graph $\mathcal{G}_{\mathcal{I}}$ and minimize the following:
\begin{equation}
    \min\limits_{\mathbf{e}_u, \mathbf{e}_j} \text{ }- \sum\limits_{(u, i) \in \mathbf{R}^{+}_s} \text{ } \sum\limits_{j \in topk(\mathbf{R}^{\mathcal{I}}_{i, *})}\frac{\mathbf{R}^{\mathcal{I}}_{i, j}}{\sigma^{\mathcal{I}}_i - \mathbf{R}^{\mathcal{I}}_{i,i}} \sqrt{\frac{\sigma^{\mathcal{I}}_i}{\sigma^{\mathcal{I}}_j}} log(sig(\mathbf{e}_u^\top \cdot \mathbf{e}_j)),
\end{equation}
where $topk()$ retrieves the top-k values of a matrix row-wise, and $\sigma_*^{\mathcal{I}}$ is the node degree calculated on $\mathcal{G}_{\mathcal{I}}$. 

\subsubsection{SVD-GCN} \citet{DBLP:conf/cikm/PengSM22} propose a reformulation of the GCN-based message-passing which leverages the similarities between graph convolutional layers and singular value decomposition (i.e., SVD). Specifically, they rewrite the message-passing introduced in LightGCN by making two aspects explicitly emerge, namely: (i) even- and odd-connection message aggregations, and (ii) singular values and vectors obtained by decomposing the user-item interaction matrix $\mathbf{R}$ through SVD. On such basis, the authors' assumption is that the traditional graph convolutional layer intrinsically learns a low-rank representation of the user-item interaction matrix where components corresponding to larger singular values tend to be enhanced. %Moreover, t
They reinterpret the over-smoothing effect as an increasing gap between singular values when stacking more and more layers. 
%In the light of this, 
The embeddings for users and items are obtained as follows:
\begin{equation}
    \mathbf{e}_u = \mathbf{p}_u exp(a_1 \boldsymbol\lambda) \cdot \mathbf{W}, \qquad
    \mathbf{e}_i = \mathbf{q}_i exp(a_1 \boldsymbol\lambda) \cdot \mathbf{W},
\end{equation}
where: (i) $\mathbf{p}_u$ and $\mathbf{q}_i$ are the left and right singular vectors of the normalized user-item interaction matrix for user $u$ and item $i$; (ii) $exp()$ is the exponential function; (iii) $a_1$ is a tunable hyper-parameter of the model; (iv) $\boldsymbol\lambda$ is the vector of the largest singular values of the normalized user-item matrix; (v) $\mathbf{W}$ is a trainable matrix to perform feature transformation. Note that the highest singular value $\lambda_{max}$ and the maximum node degree $\max(\mathcal{D})$ in the user-item interaction matrix are associated by the following inequality:
\begin{equation}
    \lambda_{max} \leq \frac{\max(\mathcal{D})}{\max(\mathcal{D}) + a_2},
\end{equation}
where $a_2$ is another tunable hyper-parameter of the model to control the gap among singular values. Similarly to UltraGCN, the authors recognize the importance of different types of relationships during the message-passing (i.e., user-item, user-user, item-item). For this reason, they decide to augment the loss function with other components addressing also the similarities among node embeddings from the same partition:
\begin{equation}
    \begin{aligned}
        \min\limits_{\mathbf{e}_v, \mathbf{e}_w, \mathbf{e}_j} \text{ }&- \sum\limits_{(v, w) \in (\mathbf{R}^{\mathcal{*}}_s)^{+}} log(sig(\mathbf{e}^\top_v \cdot \mathbf{e}_w)) \text{ }+ \\
        &- \sum\limits_{(v, j) \in (\mathbf{R}^{\mathcal{*}}_s)^{-}} log(sig(-\mathbf{e}^\top_v \cdot \mathbf{e}_j)),
    \end{aligned}
\end{equation}
where $v$, $w$, and $j$ are nodes from the same partition, and $\mathbf{R}^*$ is the interaction matrix of that partition.

\subsection{Algorithms}
\label{app:alg}
In Algorithm \ref{alg:sampling} and Algorithm \ref{alg:data-generation} we report the pseudocode to perform graph sampling and the sub-dataset generation, respectively. Note that $uniform_N()$ is the function that uniformly samples $N$ elements from a set, while $uniform()$ samples only one element from a set.

\begin{algorithm}[!t]
\caption{Graph sampling}
\label{alg:sampling}
\SetAlgoLined
\textbf{Input:} Bipartite user-item graph $\mathcal{G}$, dropout rate $\mu$, graph sampling strategy \texttt{\textit{sampling}}.\\
\textbf{Output:} Sampled graph $\mathcal{G}_m$.\\
\uIf{\texttt{sampling} $==$ \texttt{nodeDropout}}{
    %\texttt{// calculate nodes to sample according to} $d$\\
    $N = (U + I) * (1 - \mu)$ \\
    %\texttt{// sample $N$ nodes}\\
    $\mathcal{V}_m \leftarrow uniform_N(\mathcal{U} \cup \mathcal{I})$\\
    %\texttt{// mask $\mathbf{A}$ according to $\mathcal{V}_m$}\\
    $\mathbf{A}_m \leftarrow mask_{node}(\mathbf{A}, \mathcal{V}_m)$
}
\uElseIf{\texttt{sampling} $==$ \texttt{edgeDropout}}{
    %\texttt{// calculate edges to sample according to} $d$\\
    $N = E * (1 - \mu)$ \\
    %\texttt{// sample $N$ edges}\\
    $\mathcal{E}_m \leftarrow uniform_N(\mathcal{E}_{u \rightarrow i})$\\
    %\texttt{// mask $\mathbf{A}$ according to $\mathcal{E}_m$}\\
    $\mathbf{A}_m \leftarrow mask_{edge}(\mathbf{A}, \mathcal{E}_m)$\\
    %\texttt{// induce the set of nodes $\mathcal{V}_m$}\\
    $\mathcal{V}_m \leftarrow induce(\mathbf{A}_m)$
}
\phantom{ }\\
%\texttt{// induce $\mathcal{G}_m$ through $\mathcal{V}_m$ and $\mathbf{A}_m$}\\
$\mathcal{G}_m \leftarrow \{\mathcal{V}_m, \mathbf{A}_m\}$ \\
Return $\mathcal{G}_m$.
\end{algorithm}
\begin{algorithm}[!t]
\SetAlgoLined
\textbf{Input:} Bipartite user-item graph $\mathcal{G}$, number of samples $M$.\\
\textbf{Output:} $M$ sampled graphs.\\
$m \leftarrow 1$\\
$\mathcal{M} = \{\}$\\
\While{$m \leq M$}{
    % \texttt{// get dropout rate}\\
    $\mu \leftarrow uniform([0.7, 0.9])$\\
    % \texttt{// choose graph sampling strategy}\\
    $\texttt{\textit{sampling}} \leftarrow uniform(\{\texttt{nodeDropout}, \texttt{edgeDropout}\})$\\
    % \texttt{// add sampled graph to the set}\\
    $\mathcal{M} \leftarrow \mathcal{M} \cup sample(\mathcal{G}, \mu, \texttt{\textit{sampling}})$\\
    % \texttt{// increment number of generated samples}\\
    $m \leftarrow m + 1$
}
Return $\mathcal{M}$.
\caption{Sub-dataset generation.}
\label{alg:data-generation}
\end{algorithm}

\subsection{Experimental setting}
\label{app:exp_sett}

We provide here a detailed description of the experimental settings for our proposed explanatory framework. First, we present the recommendation datasets for this study. Then, we report on the adopted characteristics, along with details about their (optional) value rescaling and denomination. Finally, we describe the methodology we follow to train and evaluate the graph-based recommendation models to foster the reproducibility of this work.

\subsubsection{Recommendation datasets} We use specific versions of Yelp2018~\cite{DBLP:conf/cikm/PengSM22} and Gowalla~\cite{DBLP:conf/sigir/0001DWLZ020} (whose results are reported in the main paper), plus Amazon-Book~\cite{DBLP:conf/www/WangHWYL0C21} (whose results are only reported in this Appendix to stay within the page limits). The usage of such datasets is motivated by their popularity in graph collaborative filtering~\cite{DBLP:conf/sigir/0001DWLZ020, DBLP:conf/cikm/MaoZXLWH21, DBLP:conf/www/LinTHZ22, DBLP:conf/cikm/GongSWLL22}. Yelp2018~\cite{DBLP:journals/corr/Asghar16} collects data about users and businesses interactions, Amazon-Book is a sub-category of the Amazon dataset~\cite{DBLP:conf/www/HeM16}, and Gowalla~\cite{DBLP:conf/kdd/ChoML11} is a social-based dataset where users share their locations. Note that, to provide a coherent calculation of the characteristics, we retained only the subset of nodes and edges for each dataset which induces the widest connected graph. In the following, we present the calculation of characteristics, experimentally justifying their adoption.

\subsubsection{Characteristics calculation}
\label{app:char-calc}
Following the same setting as in~\cite{DBLP:conf/sigir/DeldjooNSM20}, we generate $M = 600$ sub-datasets from the original ones through the techniques described in Algorithm \ref{alg:sampling} and Algorithm ~\ref{alg:data-generation}, resulting in a total of 1,800 synthetic samples (if we consider all the three datasets in the main paper and in the Appendix). Second, inspired by similar works~\cite{DBLP:journals/tmis/AdomaviciusZ12, DBLP:conf/sigir/DeldjooNSM20}, we decide to apply the log10-scale to the formulation of some characteristics to obtain values within comparable order of magnitude, thus making the training of the explanatory model more stable. In Table \ref{tab:shorthand} we provide a comprehensive outlook on the set of characteristics, where we apply a renaming scheme for the sake of simple understanding and reference. Furthermore, Table \ref{tab:dataset-chars} displays the statistics of the overall datasets and the aggregated characteristics for the generated samples. Finally, Figure \ref{fig:correlation} empirically supports the usage of the selected characteristics, as they appear loosely correlated.

\begin{table}[!b]
\caption{Selected \textit{classical} and \textit{topological} characteristics. We report the full name, the symbol, whether it is rescaled via log10, and the shorthand adopted.}
\label{tab:shorthand}
% \begin{adjustbox}{width=0.8\textwidth,center}
\begin{tabular}{l|l|c|c|l}
\toprule
\multicolumn{1}{l}{\textbf{Type}} & \multicolumn{1}{l}{\textbf{Characteristics}} & \multicolumn{1}{l}{\textbf{Symbol}} & \multicolumn{1}{l}{\textbf{Log10}} & \multicolumn{1}{l}{\textbf{Shorthand}} \\
 \cmidrule{1-5}
\multirow{5}{*}{\textit{Classical}} & {Space size} & {$\zeta$} & {\checkmark} & {$SpaceSize_{log}$} \\
 & Shape & $\pi$ & \checkmark & $Shape_{log}$ \\
 & {Density} & {$\delta$} & {\checkmark} & {$Density_{log}$} \\
 & Gini user & $\kappa_{\mathcal{U}}$ &  & $Gini\text{-}U$ \\
 & {Gini item} & {$\kappa_{\mathcal{I}}$} & {} & {$Gini\text{-}I$} \\
 \hline
\multirow{6}{*}{\textit{Topological}} & {Average degree user} & {$\sigma_{\mathcal{U}}$} & {\checkmark} & {$AvgDegree\text{-}U_{log}$} \\
 & Average degree item & $\sigma_{\mathcal{I}}$ & \checkmark & $AvgDegree\text{-}I_{log}$ \\
 & {Average clustering coefficient user} & {$\gamma_{\mathcal{U}}$} & {\checkmark} & {$AvgClustC\text{-}U_{log}$} \\
 & Average clustering coefficient item & $\gamma_{\mathcal{I}}$ & \checkmark & $AvgClustC\text{-}I_{log}$ \\
 & {Degree assortativity user} & {$\rho_{\mathcal{U}}$} & {} & {$Assort\text{-}U$} \\
 & Degree assortativity item & $\rho_{\mathcal{I}}$ &  & $Assort\text{-}I$\\
\bottomrule
\end{tabular}
% \end{adjustbox}
\end{table}
\begin{table}[!b]
\caption{Dataset overall statistics and characteristic aggregated statistics (minimum and maximum values, mean, and standard deviation) on the sampled sub-datasets.}
\label{tab:dataset-chars}
% \begin{adjustbox}{width=1\textwidth,center}
    \begin{tabular}{l|cccc|cccc|cccc}
    \toprule
        \multicolumn{1}{c}{} & \multicolumn{4}{c}{\textbf{Yelp2018}} & \multicolumn{4}{c}{\textbf{Amazon-Book}} & \multicolumn{4}{c}{\textbf{Gowalla}} \\ \cmidrule{2-13}
        \multicolumn{1}{c}{} & \multicolumn{4}{c}{\makecell[c]{\textit{\ul{Overall Statistics}}\\\textbf{Users:} 25,677 \quad \textbf{Items:} 25,815\\\textbf{Interactions:} 696,865}} & \multicolumn{4}{c}{\makecell[c]{\textit{\ul{Overall Statistics}}\\\textbf{Users:} 70,679 \quad \textbf{Items:} 24,915\\\textbf{Interactions:} 846,434}} & \multicolumn{4}{c}{\makecell[c]{\textit{\ul{Overall Statistics}}\\\textbf{Users:} 29,858 \quad \textbf{Items:} 40,981\\\textbf{Interactions:} 1,027,370}} \\ \cmidrule{2-13}
        \multicolumn{1}{c}{\textbf{Characteristics}} & \textbf{Min} & \textbf{Max} & \textbf{Mean} & \multicolumn{1}{c}{\textbf{Std}} & \textbf{Min} & \multicolumn{1}{c}{\textbf{Max}} & \textbf{Mean} & \multicolumn{1}{c}{\textbf{Std}} & \textbf{Min} & \multicolumn{1}{c}{\textbf{Max}} & \textbf{Mean} & \textbf{Std} \\
        \cmidrule{1-13}  
        $SpaceSize_{log}$ & 0.256 & 1.393 & 1.000 & 0.379 & 0.405 & 1.593 & 1.176 & 0.384 & 0.430 & 1.541 & 1.161 & 0.375 \\
        $Shape_{log}$ & 0.019 & 0.105 & 0.045 & 0.014 & 0.325 & 0.443 & 0.407 & 0.021 & -0.149 & -0.097 & -0.129 & 0.008 \\ 
        $Density_{log}$ & -3.699 & -2.693 & -3.219 & 0.358 & -3.902 & -2.896 & -3.497 & 0.365 & -3.889 & -2.876 & -3.380 & 0.363 \\ 
        $Gini\text{-}U$ & 0.443 & 0.508 & 0.486 & 0.008 & 0.384 & 0.499 & 0.459 & 0.023 & 0.462 & 0.512 & 0.491 & 0.007 \\ 
        $Gini\text{-}I$ & 0.500 & 0.609 & 0.575 & 0.019 & 0.518 & 0.618 & 0.586 & 0.018 & 0.437 & 0.502 & 0.478 & 0.008 \\ 
        $AvgDegree\text{-}U_{log}$ & 0.523 & 0.926 & 0.758 & 0.110 & 0.318 & 0.609 & 0.476 & 0.077 & 0.603 & 1.017 & 0.846 & 0.115 \\ 
        $AvgDegree\text{-}I_{log}$ & 0.565 & 0.955 & 0.804 & 0.098 & 0.682 & 1.043 & 0.883 & 0.096 & 0.487 & 0.888 & 0.717 & 0.109 \\ 
        $AvgClustC\text{-}U_{log}$ & -1.144 & -0.662 & -0.947 & 0.126 & -0.757 & -0.407 & -0.602 & 0.095 & -1.211 & -0.741 & -1.013 & 0.122 \\ 
        $AvgClustC\text{-}I_{log}$ & -1.092 & -0.652 & -0.922 & 0.105 & -1.124 & -0.751 & -0.967 & 0.099 & -1.080 & -0.614 & -0.881 & 0.124 \\ 
        $Assort\text{-}U$ & -0.051 & 0.235 & 0.021 & 0.035 & -0.041 & 0.533 & 0.052 & 0.074 & 0.042 & 0.544 & 0.188 & 0.071 \\ 
        $Assort\text{-}I$ & -0.002 & 0.237 & 0.067 & 0.037 & 0.000 & 0.842 & 0.443 & 0.264 & -0.037 & 0.161 & 0.021 & 0.028 \\ \bottomrule
    \end{tabular}
    % \end{adjustbox}
\end{table}
\input{plot/correlation-heatmap}

\subsubsection{Reproducibility} We perform the random subsampling strategy to split each sub-dataset into train and test (80\% and 20\%, respectively). Then, we retain the 10\% of the train as validation for the early stopping to avoid overfitting. To train LightGCN, DGCF, UltraGCN, and SVD-GCN, we fix their configurations (i.e., hyper-parameters and patience for the early stopping) to the best values according to the original papers, since our scope is not to fine-tune them. Finally, following the literature, we use the \textit{Recall@20} calculated on the validation for the early stopping, and evaluate the models by assessing the same metric on the test set. Codes, datasets, and configuration files to reproduce all the experiments are available at this link: ~\url{https://github.com/sisinflab/Graph-Characteristics}.

\subsection{Additional results for RQ1}
\label{app:add_exp_1}
Table \ref{tab:rq1_app} reports additional results for RQ1 on Amazon-Book, when considering the \textit{Recall@20} as recommendation metric (as done in Table \ref{tab:rq1}). Conversely, Table \ref{tab:rq1_ndcg} displays additional results for RQ1 when considering all three datasets for the \textit{nDCG@20} as recommendation metric.

\begin{table}[!h]
\caption{Additional results for RQ1 on Amazon-Book. The current table is to be interpreted the same way as Table \ref{tab:rq1}.}
\label{tab:rq1_app}
% \begin{adjustbox}{width=0.6\textwidth,center}
    \centering
    \begin{tabular}{l|c|c|c|c}
    \toprule
        \multicolumn{1}{c}{\textbf{Characteristics}} & \multicolumn{1}{c}{\textbf{LightGCN}} & \multicolumn{1}{c}{\textbf{DGCF}} & \multicolumn{1}{c}{\textbf{UltraGCN}} & \multicolumn{1}{c}{\textbf{SVD-GCN}} \\ \cmidrule{1-5} 
        \rowcolor{gray} \ $R^{2}$(adj. $R^{2}$) & $0.953 (0.952)$ & $0.951 (0.950)$ & $0.800 (0.797)$& $0.964 (0.963)$
 \\ \
         $Constant$ & $0.088^{***}$&$0.079^{***}$&$0.056^{***}$&$0.112^{***}$
 \\ \
         $SpaceSize_{log}$ & $0.456^{***}$& $0.364^{***}$& $0.067^{}$& $0.433^{***}$
 \\ \
         $Shape_{log}$ &$-0.668^{***}$&$-0.598^{***}$&$-0.215^{}$&$-0.582^{***}$
 \\ \
         $Density_{log}$ & $0.546^{***}$& $0.453^{***}$& $0.141^{**}$&$0.541^{***}$
 \\ \
         $Gini\text{-}U$ &$-0.073^{}$&$-0.085^{}$&$-0.350^{**}$&$-0.042^{}$
 \\ \
         $Gini\text{-}I$ & $1.302^{***}$& $1.148^{***}$& $0.772^{***}$&$1.306^{***}$
 \\ \
         $AvgDegree\text{-}U_{log}$ &$1.336^{***}$&$1.116^{***}$&$0.316^{*}$&$1.265^{***}$
 \\ \
         $AvgDegree\text{-}I_{log}$ & $0.668^{***}$& $0.518^{***}$& $0.101^{}$& $0.683^{***}$
 \\ \
         $AvgClustC\text{-}U_{log}$ &$1.627^{***}$&$1.307^{***}$&$0.210^{}$&$1.617^{***}$
 \\ \
         $AvgClustC\text{-}I_{log}$ &$0.431^{***}$&$0.337^{***}$& $0.111^{}$& $0.354^{***}$
 \\ \
        $Assort\text{-}U$ &$0.031^{}$&$0.041^{*}$&$0.070^{***}$&$0.028^{}$
 \\ \
         $Assort\text{-}I$ &$-0.010^{}$& $-0.004^{}$& $0.025^{***}$& $-0.010^{*}$ \\ 
   \bottomrule
 \multicolumn{5}{l}{\textit{***p-value $\leq$ 0.001, **p-value $\leq$ 0.01, *p-value $\leq$ 0.05}}
    \end{tabular}
% \end{adjustbox}
\end{table}
\begin{table}[!h]
\caption{Additional results for RQ1 on Yelp2018, Gowalla, and Amazon-Book when considering the \textit{nDCG@20} as accuracy metric. The current table is to be interpreted the same way as Table \ref{tab:rq1}, but \textit{nDCG@20} is the recommendation metric this time.}
\label{tab:rq1_ndcg}
    \centering
    % \begin{adjustbox}{width=\textwidth,center}
    \begin{tabular}{l|ccc|ccc|ccc|ccc}
    \toprule
        \multicolumn{1}{c}{\multirow{2}{*}{\textbf{Characteristics}}} & \multicolumn{3}{c}{\textbf{LightGCN}} & \multicolumn{3}{c}{\textbf{DGCF}} & \multicolumn{3}{c}{\textbf{UltraGCN}} & \multicolumn{3}{c}{\textbf{SVD-GCN}} \\ \cmidrule{2-13}
        \multicolumn{1}{c}{} & \multicolumn{1}{c}{\textbf{Yelp2018}} & \textbf{Amazon-Book} & \multicolumn{1}{c}{\textbf{Gowalla}} & \textbf{Yelp2018} & \textbf{Amazon-Book} & \multicolumn{1}{c}{\textbf{Gowalla}} & \textbf{Yelp2018} & \textbf{Amazon-Book} & \multicolumn{1}{c}{\textbf{Gowalla}} & \textbf{Yelp2018} & \textbf{Amazon-Book} & \textbf{Gowalla} \\ \cmidrule{1-13}
        \rowcolor{gray} $R^{2}$(adj. $R^{2}$) & $0.971 (0.970)$& $0.947 (0.946)$& $0.978 (0.977)$& $0.972 (0.971)$& $0.945 (0.944)$& $0.980 (0.979)$& $0.966 (0.966)$& $0.748 (0.743)$& $0.865 (0.863)$& $0.982 (0.982)$& $0.958 (0.957)$& $0.980 (0.980)$ \\ \
         $Constant$ & $0.048^{***}$&$0.043^{***}$&$0.068^{***}$&$0.043^{***}$&$0.039^{***}$&$0.061^{***}$&$0.028^{***}$&$0.025^{***}$&$0.034^{***}$&$0.056^{***}$&$0.054^{***}$&$0.076^{***}$ \\ \
         $SpaceSize_{log}$ & $0.054^{***}$& $0.286^{***}$& $0.142^{***}$& $0.086^{***}$& $0.229^{***}$& $0.170^{***}$& $-0.017^{**}$& $0.054^{}$& $0.216^{***}$& $0.062^{***}$& $0.290^{***}$& $0.107^{***}$ \\ \
         $Shape_{log}$ & $-0.191^{***}$&$-0.447^{***}$&$-0.168^{*}$&$-0.185^{***}$&$-0.389^{***}$&$-0.134^{}$&$0.062^{}$&$-0.154^{}$&$-0.019^{}$&$-0.159^{**}$&$-0.417^{***}$&$-0.193^{*}$ \\ \
         $Density_{log}$ &  $0.115^{***}$& $0.332^{***}$& $0.199^{***}$& $0.140^{***}$& $0.274^{***}$& $0.218^{***}$& $0.024^{***}$& $0.090^{**}$& $0.213^{***}$& $0.131^{***}$& $0.345^{***}$& $0.172^{***}$
 \\ \
         $Gini\text{-}U$ & $0.140^{**}$&$-0.106^{}$&$-0.034^{}$&$0.046^{}$&$-0.105^{}$&$-0.085^{}$&$0.060^{}$&$-0.194^{**}$&$-0.547^{***}$&$0.050^{}$&$-0.140^{*}$&$0.012^{}$
 \\ \
         $Gini\text{-}I$ & $0.678^{***}$& $0.720^{***}$& $0.438^{***}$& $0.588^{***}$& $0.624^{***}$& $0.368^{***}$& $0.264^{***}$& $0.393^{***}$& $-0.145^{}$& $0.561^{***}$& $0.722^{***}$& $0.482^{***}$
 \\ 
         $AvgDegree\text{-}U_{log}$ & $0.264^{***}$&$0.841^{***}$&$0.425^{***}$&$0.319^{***}$&$0.698^{***}$&$0.455^{***}$&$-0.024^{}$&$0.221^{*}$&$0.439^{***}$&$0.273^{***}$&$0.843^{***}$&$0.375^{***}$
 \\ \
         $AvgDegree\text{-}I_{log}$ & $0.073^{*}$& $0.394^{***}$& $0.257^{***}$& $0.134^{***}$& $0.309^{***}$& $0.322^{***}$& $0.038^{}$& $0.068^{}$& $0.420^{***}$& $0.113^{***}$& $0.426^{***}$& $0.182^{***}$
 \\ \
         $AvgClustC\text{-}U_{log}$ & $0.405^{***}$&$1.050^{***}$&$0.514^{***}$&$0.466^{***}$&$0.843^{***}$&$0.551^{***}$&$-0.006^{}$&$0.167^{}$&$0.461^{***}$&$0.441^{***}$&$1.094^{***}$&$0.443^{***}$
 \\ \
         $AvgClustC\text{-}I_{log}$ & $0.024^{}$& $0.205^{***}$& $0.193^{}$& $0.070^{}$& $0.163^{**}$& $0.258^{**}$& $0.038^{}$& $0.062^{}$& $0.461^{***}$& $0.016^{}$& $0.174^{**}$& $0.146^{}$
 \\ \
          $Assort\text{-}U$ & $0.058^{***}$&$0.018^{}$&$0.020^{**}$&$0.055^{***}$&$0.022^{*}$&$0.014^{*}$&$0.093^{***}$&$0.045^{***}$&$0.005^{}$&$0.048^{***}$&$0.016^{}$&$0.008^{}$
 \\ \
         $Assort\text{-}I$ & $-0.029^{*}$& $-0.005^{}$& $-0.034^{}$& $-0.029^{*}$& $-0.002^{}$& $-0.046^{}$& $0.005^{}$& $0.016^{***}$& $-0.113^{***}$& $-0.028^{*}$& $-0.006^{*}$& $-0.074^{**}$
 \\ 
   \bottomrule
 \multicolumn{13}{l}{\textit{***p-value $\leq$ 0.001, **p-value $\leq$ 0.01, *p-value $\leq$ 0.05}}
    \end{tabular}
    % \end{adjustbox}
\end{table}

\subsection{Intuition for RQ2}
\label{app:intuition}

Figure \ref{fig:scale-free} displays the relation (i.e., the black points) between the probability distribution of node degrees in the original graph and their degree values on the Gowalla dataset. As evident, high-degree nodes are less popular than low-degree ones, and this resembles the tendency of real-world networks to be \textit{scale-free}~\cite{PhysRevE.67.026112}. To be more precise, the actual degree probability distribution approximates neither the \textit{power-law} (i.e., representing \textit{scale-free} networks, in green), nor the \textit{exponential} function (i.e., in red), but it would be well-approximated by a function in-between. This suggests that the high-degree nodes are even less frequent than they usually are in \textit{scale-free} networks.  

The figure helps to re-interpret the impact of node- and edge-dropout. While node-dropout works by removing nodes (and all the edges connected to them), edge-dropout eliminates edges and the consequently-disconnected nodes. Let us consider their worst-case scenarios. For node-dropout, it would be to drop many high-degree nodes from the graph. Whereas, when considering edge-dropout, it would be to drop all the edges connected to several nodes and thus disconnect them from the graph. 

This intuition drove us towards stating that, on averagely, node-dropout has the potential to drop larger portions of the user-item graph than edge-dropout. Indeed, this might undermine the goodness of the explanations produced by our explanatory framework. The assumption further motivates the strategy we adopted to generate the sub-datasets in RQ1, where we performed both node- and edge-dropout by uniformly selecting one of them for each sampled sub-dataset in order not to bias the procedure towards either node- or edge-dropout (see again Section \ref{dataset-generation}).

\input{figures/scale_free.tex}

\subsection{Additional results for RQ2}
\label{app:add_exp_2}
Table \ref{tab:rq2_app} reports additional results for RQ2. 
\begin{table}[!h]
\caption{Additional results for RQ2 on DGCF and UltraGCN. The current table is to be interpreted the same way as Table \ref{tab:rq2}.}
\label{tab:rq2_app}
% \begin{adjustbox}{width=\textwidth,center}
    \centering
    \begin{tabular}{l|cc|cc|cc|cc}
    \toprule
         \multicolumn{1}{c}{} & \multicolumn{2}{c}{\textbf{Node drop} \tikzcircle[fill=black]{2.5pt} \tikzcircle[fill=black]{2.5pt} \tikzcircle[fill=black]{2.5pt} \quad
         \textbf{Edge drop} \tikzcircle[fill=white]{2.5pt} \tikzcircle[fill=white]{2.5pt} \tikzcircle[fill=white]{2.5pt}} & \multicolumn{2}{c}{\textbf{Node drop} \tikzcircle[fill=black]{2.5pt} \tikzcircle[fill=black]{2.5pt} \tikzcircle[fill=white]{2.5pt} \quad
         \textbf{Edge drop} \tikzcircle[fill=black]{2.5pt} \tikzcircle[fill=white]{2.5pt} \tikzcircle[fill=white]{2.5pt}} & \multicolumn{2}{c}{\textbf{Node drop} \tikzcircle[fill=black]{2.5pt} \tikzcircle[fill=white]{2.5pt} \tikzcircle[fill=white]{2.5pt} \quad
         \textbf{Edge drop} \tikzcircle[fill=black]{2.5pt} \tikzcircle[fill=black]{2.5pt} \tikzcircle[fill=white]{2.5pt}} & \multicolumn{2}{c}{\textbf{Node drop} \tikzcircle[fill=white]{2.5pt} \tikzcircle[fill=white]{2.5pt} \tikzcircle[fill=white]{2.5pt} \quad
         \textbf{Edge drop} \tikzcircle[fill=black]{2.5pt} \tikzcircle[fill=black]{2.5pt} \tikzcircle[fill=black]{2.5pt}} \\ \cmidrule{2-9}
         \multicolumn{1}{c}{} & \multicolumn{2}{c}{\makecell[c]{\textit{\ul{Average Sampling Statistics}}\\\textbf{Users:} 5,828 \quad \textbf{Items:} 7,887 \\ \textbf{Interactions:} 45,620}} & \multicolumn{2}{c}{\makecell[c]{\textit{\ul{Average Sampling Statistics}}\\\textbf{Users:} 12,744 \quad \textbf{Items:} 17,229 \\ \textbf{Interactions:} 97,785}} & \multicolumn{2}{c}{\makecell[c]{\textit{\ul{Average Sampling Statistics}}\\\textbf{Users:} 21,730 \quad \textbf{Items:} 29,316 \\ \textbf{Interactions:} 160,919\\}} & \multicolumn{2}{c}{\makecell[c]{\textit{\ul{Average Sampling Statistics}}\\\textbf{Users:} 28,526 \quad \textbf{Items:} 38,467 \\ \textbf{Interactions:} 209,659}} \\ \cmidrule{2-9} 
         \multicolumn{1}{c}{\textbf{Characteristics}} & \multicolumn{1}{c}{\textbf{DGCF}} & \multicolumn{1}{c}{\textbf{UltraGCN}} & \multicolumn{1}{c}{\textbf{DGCF}} & \multicolumn{1}{c}{\textbf{UltraGCN}} & \multicolumn{1}{c}{\textbf{DGCF}} & \multicolumn{1}{c}{\textbf{DGCF}} & \multicolumn{1}{c}{\textbf{UltraGCN}} \\ 
         \cmidrule{1-9} 
         \rowcolor{gray} $R^{2}$(adj. $R^{2}$) &$0.888 (0.884)$&$0.597 (0.583)$ &$0.973 (0.972)$&$0.833 (0.827)$&$0.988 (0.988)$&$0.883 (0.879)$&$0.994 (0.994)$&$0.599 (0.584)$ \\
        $Constant$ &$0.162^{***}$&$0.091^{***}$&$0.131^{***}$&$0.074^{***}$&$0.085^{***}$&$0.051^{***}$&$0.051^{***}$&$0.034^{***}$ \\
        $SpaceSize_{log}$ &$0.130^{**}$&$0.175^{*}$&$0.192^{***}$&$0.358^{***}$&$0.264^{***}$&$0.337^{***}$&$-0.188^{***}$&$1.644^{***}$ \\
        $Shape_{log}$ &$-0.109^{}$&$-0.096^{}$&$-0.232^{*}$&$-0.022^{}$&$-0.136^{}$&$-0.029^{}$&$-0.011^{}$&$1.055^{**}$ \\
        $Density_{log}$ &$-0.005^{}$&$0.394^{***}$&$0.294^{***}$&$0.355^{***}$&$0.351^{***}$&$0.340^{***}$&$0.168^{***}$&$0.185^{}$ \\
        $Gini\text{-}U$ &$-0.136^{}$&$-0.824^{***}$&$0.083^{}$&$-0.880^{***}$&$0.130^{}$&$-0.775^{**}$&$0.200^{*}$&$-0.961^{}$ \\
        $Gini\text{-}I$ &$0.756^{***}$&$-0.152^{}$&$0.717^{***}$&$-0.248^{}$&$0.668^{***}$&$-0.333^{}$&$0.264^{**}$&$-0.732^{}$ \\
        $AvgDegree\text{-}U_{log}$ &$0.179^{**}$&$0.617^{***}$&$0.601^{***}$&$0.723^{***}$&$0.684^{***}$&$0.692^{***}$&$-0.014^{}$&$1.302^{***}$\\
        $AvgDegree\text{-}I_{log}$ &$0.070^{}$&$0.521^{**}$&$0.369^{***}$&$0.702^{***}$&$0.547^{***}$&$0.663^{***}$&$-0.025^{}$&$2.356^{***}$ \\
        $AvgClustC\text{-}U_{log}$ &$0.362^{***}$&$0.619^{**}$&$0.715^{***}$&$0.641^{**}$&$0.706^{***}$&$0.481^{}$&$0.001^{}$&$1.099^{**}$\\
        $AvgClustC\text{-}I_{log}$ &$-0.080^{}$&$0.412^{}$&$0.252^{}$&$0.903^{**}$&$0.571^{**}$&$0.962^{**}$&$-0.083^{}$&$2.415^{***}$ \\
        $Assort\text{-}U$ &$-0.001^{}$&$0.001^{}$&$0.011^{}$&$0.000^{}$&$0.001^{}$&$0.012^{}$&$0.008^{}$&$0.064^{}$ \\
        $Assort\text{-}I$ &$-0.050^{}$&$-0.111^{**}$&$0.002^{}$&$-0.151^{**}$&$0.002^{}$&$-0.086^{}$&$-0.032^{}$&$-0.141^{}$
         \\
    \bottomrule
    \multicolumn{9}{l}{\textit{***p-value $\leq$ 0.001, **p-value $\leq$ 0.01, *p-value $\leq$ 0.05}}
    \end{tabular}
    % \end{adjustbox}
\end{table}
